# Supplementary material for: Designing Long-term Group Fair Policies in Dynamical Systems
Source: arXiv:2311.12447 source file (2023-11-21)
Supplement: Supplementary file 1 [file 95_Appendix_Results-Gen2.tex]

%%%%%%%%%%%%%%%%%%%%%%%%%%%%%%%
\section{Results for Additional Example}
%%%%%%%%%%%%%%%%%%%%%%%%%%%%%%%

\todo{Add}
