# Supplementary material for: Designing Long-term Group Fair Policies in Dynamical Systems
Source: arXiv:2311.12447 source file (2023-11-21)
Supplement: Supplementary file 2 [file dynamics-s.tex]

  \begin{tikzpicture}[every node/.style={inner sep=0,outer sep=0}]

        \node[state, fill=gray!60] (x0) at (0,0) {$S_0$};
        \node[state, fill=gray!60] (x1) [right  =  2  cm of x0]  {$S_1$};
        \node[state, fill=gray!60] (x2) [right  =  2 cm of x1]  {$S_2$};
        % \node[state, fill=gray!60] (s) [above  =  0.6cm of x1]  {$S$};
         \node[state, fill=gray!60] (y0) [below  =  0.6 cm of x0] {$X_0$};
        \node[state, fill=gray!60] (y1) [below  =  0.6 cm of x1]  {$X_1$};
        \node[state, fill=gray!60] (y2) [below  =  0.6 cm of x2]  {$X_2$};
        \node[state, fill=gray!60] (s0) [right  =  0.3 cm of y0] {$Y_0$};
        \node[state, fill=gray!60] (s1) [right  =  0.6 cm of y1]  {$Y_1$};
        \node[state, fill=gray!60] (s2) [right  =  0.6 cm of y2]  {$Y_2$};
        \node[state,  fill=gray!60] (d0) [below  =  0.6 cm of s0] {$D_0$};
        \node[state,  fill=gray!60] (d1) [below  =  0.6 cm of s1]  {$D_1$};
        \node[state,  fill=gray!60] (d2) [below  =  0.6 cm of s2]  {$D_2$};

        % \path (x0) edge [thick, color=blue!60](x1);
        % \path (x1) edge [thick, color=blue!60] (x2);
        \path (x0) edge [thick](x1);
        \path (x1) edge [thick] (x2);
        
        % \path (s) edge [thick](y0);
        % \draw [thick, ->] (s) to [out=250,in=120] (y1);
        % \path (s) edge [thick](y2);

        % \path (s) edge [thick](d0);
        % \draw [thick, ->] (s) to [out=290,in=65] (d1);
        % \path (s) edge [thick](d2);

        % \path (s) edge [thick](x0);
        % \path (s) edge [thick](x1);
        % \path (s) edge [thick](x2);

        \path (x0) edge [thick](y0);
        \path (x1) edge [thick](y1);
        \path (x2) edge [thick](y2);

        \path (x0) edge [thick](s0);
        \path (x1) edge [thick](s1);
        \path (x2) edge [thick](s2);

        \path (s0) edge [thick](x1);
        \path (s1) edge [thick](x2);
        % \path (s2) edge [thick](x2);

        % \draw [thick, ->] (y0) to [out=300,in=75] (d0);
        % \draw [thick, ->] (y1) to [out=300,in=75] (d1);
        % \draw [thick, ->] (y2) to [out=300,in=75] (d2);
        \path  (y0) edge [thick] (d0);
        \path  (y1) edge [thick] (d1);
        \path   (y2) edge [thick] (d2);
        
        % \path (x0) edge [thick](d0);
        % \path (x1) edge [thick](d1);
        % \path (x2) edge [thick](d2);

        % \path (d0) edge [thick, color=blue!60](x1);
        % \path (d1) edge [thick, color=blue!60](x2);

        % \path (y0) edge [thick, color=blue!60](x1);
        % \path (y1) edge [thick, color=blue!60](x2);
        \path (d0) edge [thick](x1);
        \path (d1) edge [thick](x2);

        % \path (y0) edge [thick](x1);
        % \path (y1) edge [thick](x2);


\end{tikzpicture}

  
